# Supplementary material for: On the Parallel Reconstruction from Pooled Data
Source: arXiv:1905.01458 source file (2022-04-13)
Supplement: Supplementary file 1 [file 90-appendix.tex]

\let\section\subsection
\let\subsection\paragraph

\section{Preliminaries}\label{A_Prel}
In this appendix we present some standard results on concentration bounds and comparison of distributions. Afterwards, we present some technical lemmas from the theory of concentration inequalities of the binomial distribution and approximating results for random walks that are used throughout the paper.

We begin, for the convenience of the reader, with the basic Chernoff bound in the form which we will employ due to \cite{Asymptopia}. 
\begin{lemma}\label{Lem_ChernoffBoundDKL}
Let $X \sim \Bin(n, p), \epsilon > 0$ and $\delta \in (0,1)$. Then
  \begin{align*}
      \Pr \brk{ X > (1+\delta)np} &\leq \exp \bc{ - np \delta^2 / (2 + \delta) } \intertext{and}
      \Pr \brk{ X < (1-\delta)np} &\leq \exp \bc{ - np \delta^2 / 2 }.
  \end{align*}
\end{lemma}

The following lemmas are results on the asymptotic behavior of random walks. A random walk $\vec R$ can be described by its transition probabilities $R(x,y)$. The simple random walk on $\ZZ$ has the transition probabilities $R(x, x+1) = R(x,x-1) = 1/2.$
\begin{lemma}[Section 1.5 of \cite{Asymptopia}]\label{randomwalk}
The probability that a one-dimensional simple random walk with $2j$ steps will end at its original position is asymptotically given by $(\pi j)^{-1/2}(1+O(j^{-1}))$.
\end{lemma}

\begin{lemma}\label{binomial}
The following asymptotic equivalence holds for every $0 < p = p(n) < 1$ s.t.\ $np \to \infty$.
\begin{align}
    \MoveEqLeft \sum_{j=1}^{n/2} \binom{n}{2j}p^{2j}(1-p)^{n-2j}j^{-1/2} \label{Eq_AsympEquivalenceHalfBinomialRoot} \\\notag
    &= 2^{-1/2} \sum_{j=1}^n \binom{n}{j} p^{j}(1-p)^{n-j} j^{-1/2} + O( (np)^{-1} )
\end{align}
\end{lemma}

\begin{proof}
Let $\vX \sim \Bin_{\geq 1}(n, p)$ and define $a_j = \Pr \bc{\vX = j} / \sqrt{j/2}$ for $j=1 \dots n$. Then $$a_{j+1}/a_j = \bc{p/(1-p)}\bc{j / (j+1)^3}^{1/2} \bc{n - j}$$ is larger than $1$ up to $j^{\star} \in \cbc{ \floor{(n+1)p}, \floor{(n+1)p -1}}$, depending on $n$ being even or odd, and strictly less than $1$ for $j = j^{\star}+1,...,n$. Furthermore, $a_j = o(1)$ for every $j$. Define $j'$ as the largest even integer s.t.\ $ j' \leq j^{\star}$. Then 
\begin{align}
    \sum_{j = 1}^{n/2} a_{2j} & \geq \frac{1}{2} \bc{\sum_{j = 1}^{j'/2} a_{2j} + a_{2j -1} + \sum_{j = j'/2 + 1}^{n/2 - 1} a_{2j} + a_{2j + 1}} \notag \\
    &= \bc{ \frac{1}{2} \sum_{j=1}^n a_j} + \frac{1}{2}\bc{ a_{j'+1} + a_n + a_{n-1}\cdot \vecone{ ( n \text{ odd } ) }} \notag \\
    &= \bc{ \frac{1}{2} \sum_{j=1}^n a_j} + O((np)^{-2}), \label{Eq_HalfBinomialUpper}
\end{align}
and similarly
\begin{align}
    \sum_{j = 1}^{n/2} a_{2j} &\leq \frac{1}{2} \bc{\sum_{j = 1}^{j'/2} a_{2j} + a_{2j + 1} + \sum_{j = j'/2 + 1}^{n/2 - 1} a_{2j - 1} + a_{2j}} \notag\\
    &\leq \bc{ \frac{1}{2} \sum_{j=1}^n a_j} + O((np)^{-2}). \label{Eq_HalfBinomialLower}
\end{align}
Together, \cref{Eq_HalfBinomialUpper,Eq_HalfBinomialLower} imply \eqref{Eq_AsympEquivalenceHalfBinomialRoot}. 
\end{proof}

Beside these purely combinatorial standard results, we require to bound the distance between differently distributed random variables. To this end, let $\mu$ be a probability distribution over the reals, $f$ a real-valued function and $\vX \sim \mu$. Then the \emph{Jensen gap} $\cJ(f, \mu)$ is defined as $$\cJ(f, \mu) = \abs{ \Erw \brk{f(\vX)} - {f \bc{ \Erw \brk{ \vX } } } }.$$ A well known upper bound on the Jensen gap for functions $f:I \to \RR$ s.t.\ $\abs{{f(x)}- f(\Erw{[\vX]})} \leq M \abs{x - \Erw[\vX]}$ for all $x \in I$ (see equation (1.1) of \cite{gao_2018}) is given by 
\begin{align}
    \cJ(f, \mu) \leq M \Erw \brk{\abs{ \vX - \Erw{[\vX]} }}.\label{Eq_JensenGap}
\end{align}
An immediate consequence is the following corollary.
\begin{corollary}\label{Cor_JensenGap}
Let $\vX \sim \Bin_{x \geq 1}(n,p)$ be a binomial random variable conditioned on being at least 1, s.t.\ $\lim_{n \to \infty} np = \infty$.  Then, as $n \to \infty$, the following holds.
\begin{align*}
    \Erw\left[ \vX^{- 1/2} \right] = \bc{ 1 + o(n^{-1}) } {\Erw[\vX]}^{-1/2} \intertext{and} \Erw\left[ \vX^{- 1} \right] = \bc{ 1 + o(n^{-1}) } {\Erw[\vX]}^{-1}
\end{align*}
\end{corollary}
\begin{proof}Let $\vX' \sim \Bin(n,p)$. As $\Pr \bc{\vX = 0} = (1-p)^n = o(1),$ we find $\TV{\vX - \vX'} = o(1).$ Then
\cref{Lem_ChernoffBoundDKL} and \eqref{Eq_JensenGap} imply 
\begin{align}
    \abs{\Erw\left[ \vX^{- 1/2} \right] - {\Erw[\vX]}^{-1/2} } \leq \Erw \brk{\abs{ \vX - \Erw{ \brk{\vX } }} } &= o(n^{-1})  \intertext{and}
    \abs{\Erw\left[ \vX^{- 1} \right] - {\Erw[\vX ]}^{-1} } \leq \Erw \brk{\abs{ \vX - \Erw{ \brk{\vX } }}} &= o(n^{-1}). \label{Eq_JensenGap2}
\end{align}
The corollary follows directly from \cref{Eq_JensenGap2}.
\end{proof}

\iffalse
Finally, we require the following result for the balls-into-bins experiment.
\begin{lemma} \label{Lem_BallsBins}
Suppose that $B$ balls are thrown uniformly at random into $D$ bins. Then, with probability $\bc{ 1 - \bc{1 - \frac{1}{D}}^B }^D$, we find no empty bins. 
\end{lemma}
\fi

\section{Properties of the Pooling Scheme}
We now derive concentration results for the random regular pooling design. The proofs are straight-forward applications of well-known concentration inequalities discussed above.

\label{proof_properties_pooling_scheme}
The structure of the pooling scheme $\G$ is induced by its degree sequences $\vec{\Delta}=(\vec{\Delta}_i)_{i\in [n]}$ and $\Gamma$ and the specific instance of the pooling scheme is randomized. In order to prove that the event $\cR$ has really high probability (\cref{lem_event_R_high_prob}), we show each of the two statements.

\begin{lemma}\label{deltaminmax}
With probability $1-o\bc{n^{-2}}$ we have for all $i \in [n]$
\begin{align*}
   \vec{\Delta}_i &= \frac m2 + O\bc{\sqrt{m} \log n}.
\end{align*}
\end{lemma}
\begin{proof}
From the construction of $\G$, it follows that $\vec{\Delta}_i$ is distributed as $\Bin(mn/2, 1/n)$. Then \cref{Lem_ChernoffBoundDKL} implies for any $x_i (i = 1 \ldots n)$ that
\begin{align*}
   \Pr \bc{\vec{\Delta}_i > m/2 + O\bc{\sqrt{m} \log^2 n}} = n^{-\omega(1)}
\end{align*}
Taking the union bound over all $n$ entries implies the lemma.
\end{proof}

\begin{lemma}\label{deltastarminmax}
With probability $1-o\bc{n^{-2}}$ we have for all $i \in [n]$
\begin{align*}
   \vec{\Delta}^\star_i &= \bc{1-1/\sqrt{e}} m + O\bc{\sqrt{m} \log n}.
\end{align*}
\end{lemma}

\begin{proof}
The probability that an entry $x_i$ is contained in a specific query $a_j$ is given by
\begin{align*}
    p = 1 - \bc{1 - \frac{1}{n}}^{\Gamma} = \bc{1+n^{-\Omega(1)}} \bc{1 - 1/\sqrt{e}}.
\end{align*}
Since queries select their participating entries independently of each other, we observe that $\vec{\Delta}^\star_i \sim \Bin \bc{m, p}$. Thus, a standard application of the Chernoff bound and the union bound over all $n$ entries implies the lemma. 
\end{proof}

Those results suffice in order to show that $\cR$ as given through \cref{lem_event_R_high_prob} is, indeed, a high probability event.
\begin{proof}[Proof of \cref{lem_event_R_high_prob}]
The lemma follows from \cref{deltaminmax,deltastarminmax}.
\end{proof}

\section{Proof of \cref{Thm_inf}}\label{A_ITupper} 
This appendix contains the omitted proof details of the information-theoretic upper bound.
\begin{proof}[Proof of \cref{small_overlap_part_function_simplify}]
Let $\vX \sim \Bin_{\geq 1}(\Gamma, 2 (1 - \ell/k)k/n)$. Then \cref{small_overlap_part_function,Cor_JensenGap} imply
\begin{align}\label{expectation_upper}
    \MoveEqLeft \Erw[Z_{k,\ell}(\G,\vec{y})\mid \cR]\\ &\leq (1 + O(1)) \binom{k}{\ell} \binom{n-k}{k-\ell} \left(2 \pi \Erw[\vec{X}] \right)^{-m/2} .
\end{align}
In the following we use the well known fact \cite{Asymptopia}
that as $n\to\infty$ we have 
\begin{align*}
n^{-1} \log \binom{n}{np} \to H(p),
\end{align*}
where the expression $H(a)$ with $a\in[0,1]$ denotes the entropy of a $\mathrm{Be}(a)$-variable such that $H(a)=-a\log (a)-(1-a) \log (1-a)$.
We apply the $\log(\cdot)$ to \eqref{expectation_upper} and scale it with $1/n$ to get
\begin{align*}
    \MoveEqLeft \frac{1}{n}  \log\left(\Erw\left[Z_{k,\ell}(\G,\vec{y})\mid \cR  \right]\right)\notag \\
    &= \frac{1}{n} \Bigg( \log( 1+O(1) ) + \log\left(\binom{k}{\ell}\right)+\log\left(\binom{n-k}{k-\ell}\right) \notag\\
    &\quad-\frac{m}{2} \log( 2 \pi \Erw [\vec{X}])\Bigg) \notag\\
    & \leq (1+o(1)) \Bigg(\frac kn H\left(\frac \ell k\right)+ \bc{1-\frac kn} H\bc{\frac{k-\ell}{n-k}} \notag\\
    &\quad-\frac {m}{2n} \log\bc{4  \pi \Gamma \bc{1-\frac \ell k}\frac kn }\Bigg) \notag\\
    &= (1+o(1))\Bigg(\frac kn H\bc{\frac \ell k}+\bc{1-\frac kn} H\bc{\frac{k-\ell}{n-k}} \notag\\
    &\quad-\frac{c k/n \log (n/k)}{2 \log k} \log\bc{2 \pi k \bc{1- \ell/k}}\Bigg).
    \qedhere
\end{align*}
\end{proof}

\begin{proof}[Proof of \cref{Lem_small_overlap_partition_function_negative}]
Recall that for $\gamma = 1 - \exp(-1/2)$ and a constant $c$ we have 
\begin{align}
    \label{eq_recall} m = c k \log \bc{\frac {n}{k}} / \log k = c \frac{1 - \theta}{\theta} k \quad \text{and} \quad 0 \leq \ell \leq k - \gamma \log k. 
\end{align}
Then define $f_{n,k}: [0, k - \gamma \log k] \to \RR$ as
\begin{align}
 \ell \mapsto \Bigg(\frac kn H\bc{\frac \ell k}+\bc{1-\frac kn} H\bc{\frac{k-\ell}{n-k}}\notag\\-\frac{c k/n \log (n/k)}{2 \log k} \log(2 \pi (1-\ell/k)k )\Bigg) \label{func_f}
\end{align}
and assume, as usual, $0 \log 0 = 0$.
By \cref{small_overlap_part_function_simplify} we get $n^{-1} \log\left(\Erw\left[Z_{k,\ell}(\G,\vec{y})\mid \G \right]\right) \leq (1 + o(1)) f_{n,k}(\ell).$ Expanding the entropy yields
\begin{align*}
    & f_{n,k}(\ell) \\
    &=\frac 1n \Bigg(-\ell \log\bc{\frac \ell k} -\bc{k-\ell}\log\bc{1-\frac \ell k}\\
    &\quad-\bc{k-\ell} \log\bc{\frac{k-\ell}{n-k}}-\bc{n-2k+\ell} \log \bc{1-\frac{k-\ell}{n-k}}\\
    &\quad +\frac{c k \log (k/n)}{2 \log k} \log \bc{2 \pi k\bc{1-\frac \ell k}}\Bigg).
\end{align*}
Therefore,
\begin{align*}
    & f'_{n,k}(\ell) \\ &= \frac 1 n \Bigg(-\log \bc{\frac \ell k} + \log\bc{1-\frac \ell k} \\
    &\quad+ \log \bc{\frac{k-\ell}{n-k}}-\log\bc{1-\frac{k-\ell}{n-k}}-\frac{c k \log(k/n)}{2 (k-\ell) \log k }  \Bigg), \\
    & f''_{n,k}(\ell)\\
    &= \frac 1 n \Bigg(-\frac 1\ell -\frac{2}{k-\ell}-\frac{1}{n-2k+\ell} - \frac{c k \log(k/n)}{2 \log k (k-\ell)^2} \Bigg). \notag
\end{align*}
As long as $\ell = o(k)$ we get
\begin{align}
    &\label{eq_scnd_der} n f_{n,k}''(\ell) = \notag\\
    &- \frac{1}{\ell} - \frac{1}{n - 2k + \ell} - \frac{1}{k - \ell} \bc{ 2 - \frac{c k (1 - \theta)}{2 \theta (k - \ell)} } < 0
\end{align}
as $\abs{\frac{1}{k - \ell} \bc{ 2 - \frac{c k (1 - \theta)}{2 \theta (k - \ell)} }} \ll \frac{1}{\ell}$.
In this case, \cref{eq_scnd_der} shows that $f_{n,k}'$ is monotonically decreasing in $\ell$ for large enough $n$. Furthermore, $f_{n,k}'$ is continuous on $(0,  k - \gamma \log k]$. Let $\tilde c > 0$ be an arbitrary constant, then we have%\leq
\begin{align}
    & n f_{n,k}' \bc{\tilde c \frac{k^2}{n}} \notag \\ &= - \log \bc{\tilde c \frac{k}{n}} + \log \bc{ 1 - \tilde c \frac{k}{n}} + \log \bc{ \frac{k}{n} } + \log \bc{ \frac{1 - \tilde c k/n}{1 - k/n} }\notag\\
    & \quad - \log \bc{ 1 - \frac{k(1 - \tilde c k/n)}{n(1 - k/n)} } + \frac{c (1-\theta)}{2 \theta (1 - \tilde c k/n)} \label{eq_first_der} \notag \\
     & =- \log \bc{ \tilde c } + \frac{c (1 - \theta)}{\theta} + o(1) 
\end{align}
Thus, \cref{eq_first_der} implies that there are constants $0 < \tilde c_1 < \tilde c_2 < \infty$ such that 
$$ n f_{n,k}' \bc{\tilde c_1 \frac{k^2}{n}} > 0 \quad \text{and} \quad n f' \bc{\tilde c_2 \frac{k^2}{n}} < 0.$$
By the intermediate value theorem we conclude that there is $\hat c \in [\tilde c_1, \tilde c_2]$ such that $\hat c \frac{k^2}{n}$ is the unique zero of $f_{n,k}'$ for all $\ell = o(k)$ and, respectively, the unique maximizer of $f_{n,k}$ in this regime. Finally, by putting this value into \cref{func_f} we find that the highest order terms satisfy
\begin{align}
    \MoveEqLeft n f_{n,k}\bc{ \hat c \frac{k^2}{n} } < 0 \notag \\
    &\Longleftrightarrow nH\bc{k/n} - \frac{ck \log(n/k)}{2} < 0 \notag \\
    &\Longleftrightarrow     c > -2\frac{H(k/n)}{k/n \log (k/n)} = 2 + o(1). \label{eq_cond_c}
\end{align}

We are left to show that, for large enough $n$, we have $f_{n,k}(\ell) < 0 $ for any $k - \gamma \log k \geq \ell = \Theta(k)$. It is immediate from the definition that, in this case, we find
\begin{align}
    \label{eq_linear} n f_{n,k}(\ell) = - \frac{c (1 - \theta)}{2 \theta} k \log (k) + O(k)
\end{align}
which is negative.
%\todo{Oli: du hast hier doch mit Bilal lange gerechnet, wo man worauf aufpassen muss... ist das hier alles gut genug erklärt?Ja hatte ich, die Probleme waren bei unserem Modell unproblematisch}
Therefore, the lemma follows from \cref{eq_recall,eq_cond_c,eq_linear}
\end{proof}
